# Supplementary material for: Colored Noise Injection for Training Adversarially Robust Neural Networks
Source: arXiv:2003.02188 source file (2020-03-20)
Supplement: Supplementary file 1 [file 060_appendix.tex]

\section{More results}
